# Supplementary material for: Fast Optimal Locally Private Mean Estimation via Random Projections
Source: arXiv:2306.04444 source file (2023-06-26)
Supplement: Supplementary file 3 [file appendix-experiments.tex]

\section{Additional plots for the MNIST experiment}
\label{sec:apdx-exp}
We present additional details for the MNIST experiment including the description of the neural network (\Cref{tab:conv}) and additional plots with different values of the privacy parameters for the MNIST experiment. In~\Cref{fig:mnist-apdx}, we present more plots for the MNIST experiment where we train models with several privacy parameters $\diffp \in \{4,10,16\}$.

% \begin{figure*}[t]
%   \begin{center}
%     \begin{tabular}{cc}
%       \begin{overpic}[width=.45\columnwidth]{%,grid]{
%       {plots/time-comparison_eps_10}.pdf}
%       \end{overpic} &
%       \hspace{-1cm}
%       \begin{overpic}[width=.45\columnwidth]{%,grid]{
%     {plots/time-comparison_eps_16}.pdf}
%       \end{overpic}  \\
%       (a) & (b)
%     \end{tabular}
%     \caption{\label{fig:time} Run-time (in seconds) as a function of the dimension for (a) $\diffp = 10$ and (b) $\diffp = 16$.}
%   \end{center}
% \end{figure*}

\begin{figure*}[t]
  \begin{center}
    \begin{tabular}{ccc}
      \begin{overpic}[width=.35\columnwidth]{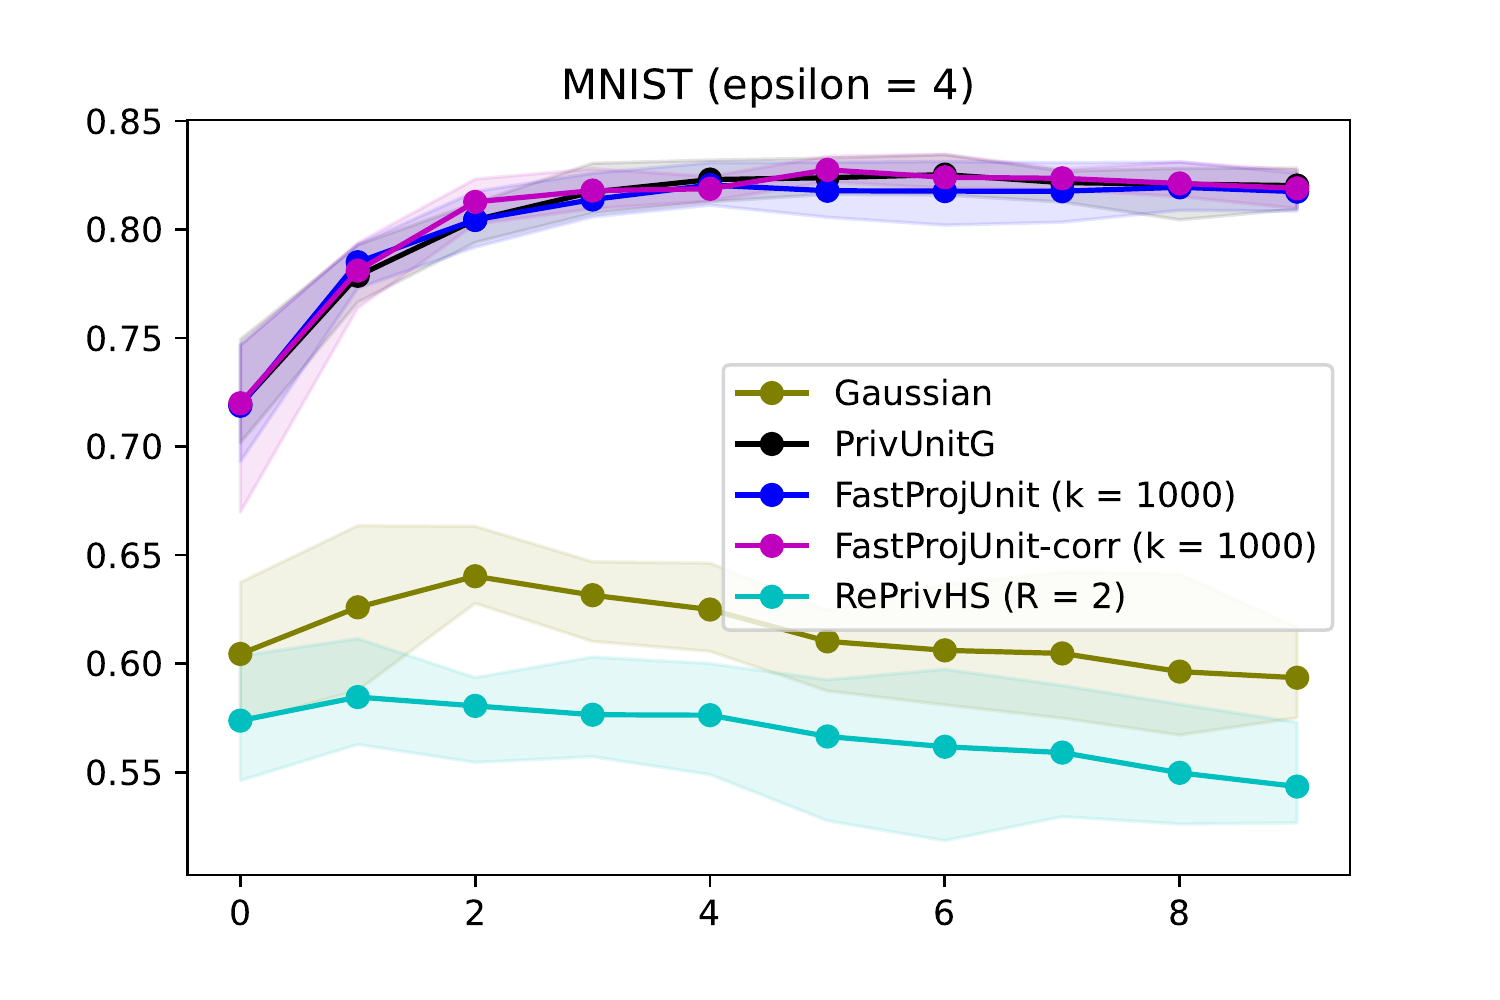}
      \end{overpic} &
      \hspace{-1cm}
      \begin{overpic}[width=.35\columnwidth]{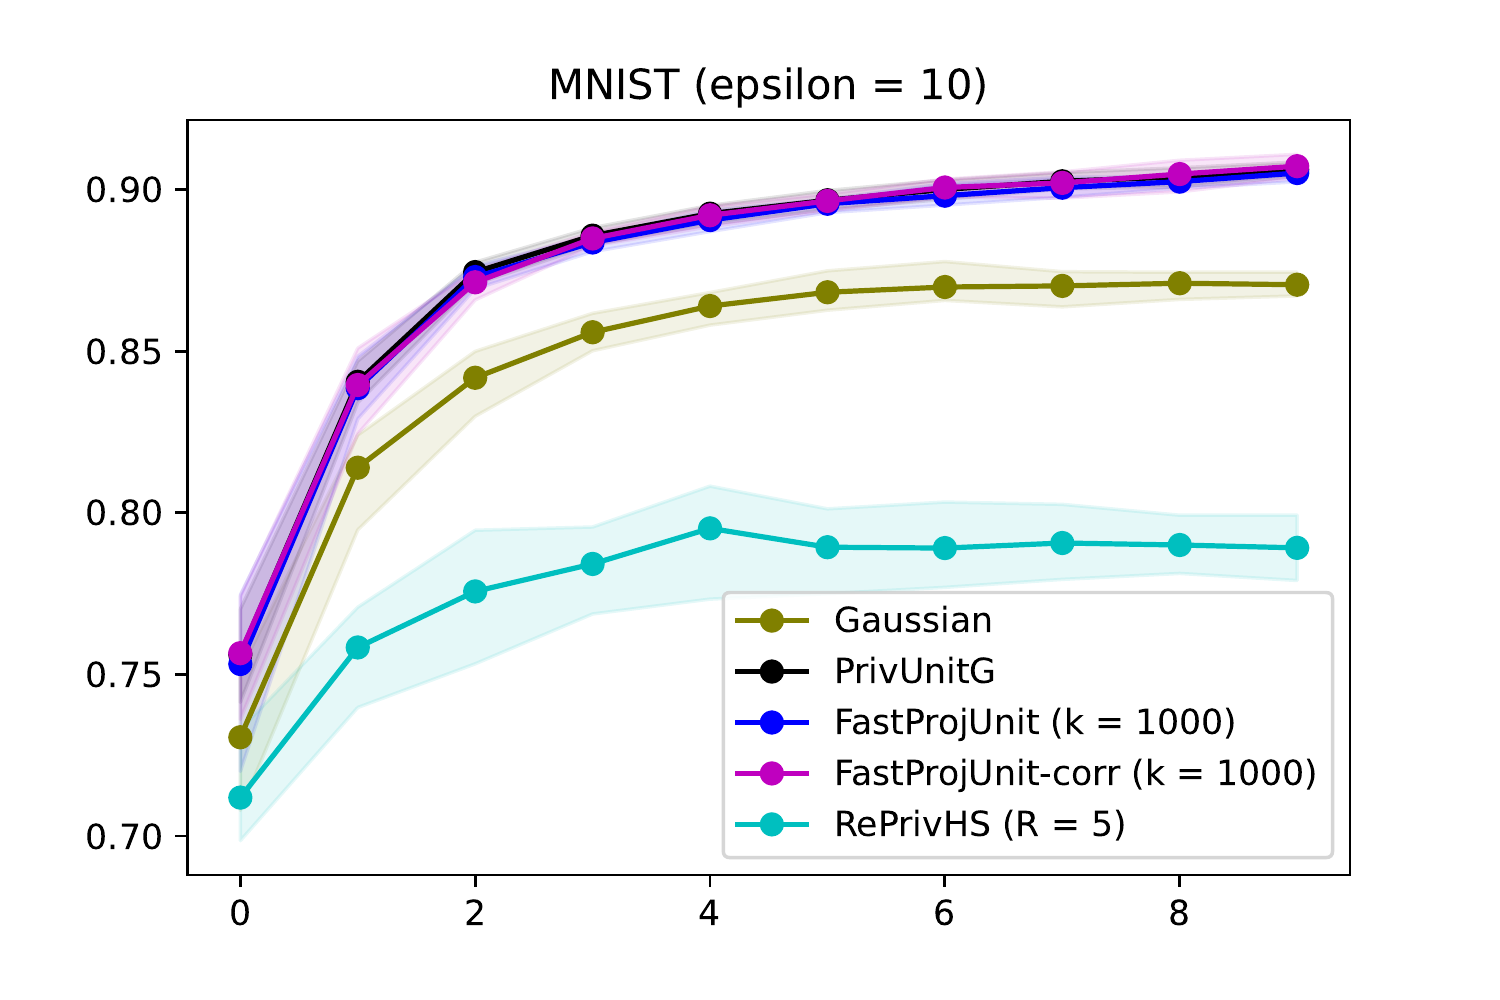}
      \end{overpic}  &
      \hspace{-1cm}
      \begin{overpic}[width=.35\columnwidth]{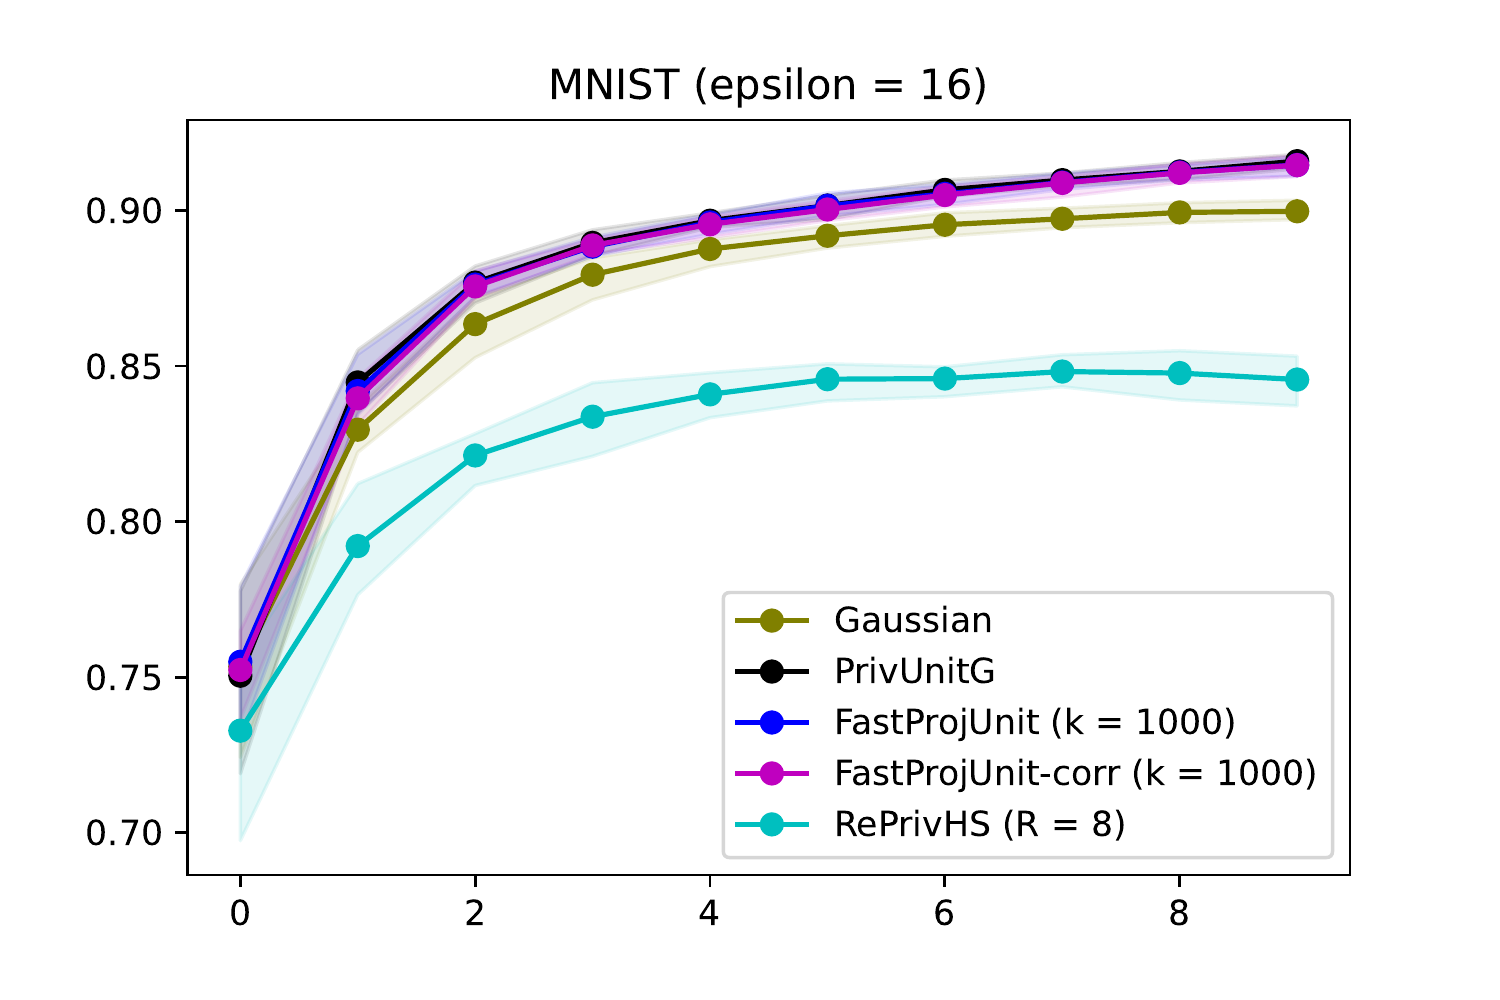}
      \end{overpic}  \\
      (a) & (b) & (c)
    \end{tabular}
    \caption{\label{fig:mnist-apdx} Test accuracy on the MNIST dataset as a function of epoch for (a) $\diffp = 4.0$, (b) $\diffp = 10.0$ and (c) $\diffp = 16.0$.}
  \end{center}
\end{figure*}

%\renewcolumntype{x}[1]{%
%	>{\raggedleft\hspace{0pt}}p{#1}}%
\begin{table}[h]
\begin{center}
\begin{tabular}{ll}
            \hline
            \textbf{Layer} & \textbf{Parameters} \\
            \hline
            Convolution $+\tanh$ & 16 filters of $8 \times 8$, stride 2, padding 2 \\
            Average pooling & $2 \times 2$, stride 1 \\
            Convolution $+\tanh$ & 32 filters of $4 \times 4$, stride 2, padding 0 \\
            Average pooling & $2 \times 2$, stride 1 \\
            Fully connected $+\tanh$ & 32 units \\
            Fully connected $+\tanh$ & 10 units \\
            \hline
\end{tabular}
\end{center}
\caption{Architecture for convolutional network model.}
\label{tab:conv}
\end{table}
